# Supplementary material for: Rheology of human blood plasma: Viscoelastic versus Newtonian behavior
Source: arXiv:1302.4102 source file (2013-02-17)
Supplement: Supplementary file 1 [file SM.pdf]

Supplementary material to the Letter

# Rheology of human blood plasma: Viscoelastic versus Newtonian behavior

by M. Brust, C. Schaefer, R. Doerr, L. Pan, M. Garcia, P. E. Arratia, and C. Wagner

## Viscoelastic instabilities of plasma, blood and replacement solutions

In order to evaluate the effects of the apparent viscoelasticity of blood plasma on the flow stability in capillaries, we investigate the flow field of plasma, PEO solutions, and RBC suspension fluids in a microfluidic contraction flow. The characteristics of the viscoelastic contraction flow with regard to the onset of (inertial-)elastic instabilities and its corresponding patterns can be described in terms of the dimensionless elasticity number $El = Wi/Re = \lambda\eta_0/(\rho D_h^2)$ [1,2]. It compares the Weissenberg number $Wi = \lambda\dot{\gamma} = \lambda V/D_h$ to the Reynolds number $Re = \rho V\, D_h/\eta_0$ and thus reflects the relative importance of elastic to inertial time scales; here *V* is the mean flow velocity, $\rho$ the fluid density and $\eta_0$ the zero shear rate viscosity. For a rectangular channel with height *h* and width *w,* the hydraulic diameter $D_h = 2wh/(w+h)$ gives an appropriate length scale of the contraction. Thus, the elasticity number *El* is constant for a given fluid in a given geometry and does not depend on the mean flow velocity *V*. According to the work of Rodd et al. [1,2] the control parameter for the onset of an instability upstream of the contraction is the Weissenberg number whereat the elasticity number gives information about the appearance of the instability. Another important parameter for the onset of an instability is the contraction ratio [3,4] which was always the same (1:16) in our case .

The microchannels are made of PDMS using standard soft lithography. Their length, width and depth are *L* = 30 mm, *W* = 40 $\mu$m, and *h* = 50 $\mu$m. These rectangular microchannels exhibit a sharp contraction of reduced width *w* = 25 $\mu$m and length *l* = 100 $\mu$m in the middle. The solutions are pushed through the channels using a syringe pump (neMESYS, Cetoni, Germany) at constant flow rates. In order to visualize the main flow patterns, fluorescent beads (0.025wt%, 500 nm) are added to the fluid. We focus on the flow directly upstream from the contraction and the particles are observed using a microscope (TE2000, Nikon) through a 20x air objective and a CCD camera (Cascade 512 F, Photometrics).

For the pure plasma, we do not observe any vortices at the entry of the contraction of the channel (Figure 1) up to shear rates of $\dot{\gamma}$~850 $10^3$ $s^{-1}$ (Wi = 730, El = 4.0, Q = 833 µl/min). The plasma flow streaklines are identical to those of pure water (not shown). A similar result is obtained for the lower concentration PEO solution ($PEO50_{15/85}$, El = 2.8) that had very comparable rheological properties to the plasma and for which we find no evidence of flow instabilities up to $\dot{\gamma}$~ 700 $10^3$ $s^{-1}$(Wi = 581, Q = 667 µl/min). However, elastic instabilities are observed for solutions with higher amount of polymer ($PEO500_{15/85}$, El = 27.3) or glycerol ($PEO50_{55/45}$, El = 42.7) concentrations.

Next, we test whether a similar instability can be observed by the addition of red blood cells to the plasma replacement solution using the 50vol% RBC solutions, namely $PBS_{15/85\text{-}Hct50}$ and $PEO50_{15/85\text{-}Hct50}$ at El = 10.8. We find that for the $PBS_{15/85\text{-}Hct50}$ no upstream vortices are observed even though RBCs are present, but the addition of only 50 ppm of PEO to the $PBS_{15/85\text{-}Hct50}$ fluid causes the upstream vortices to appear at a shear rate of $\dot{\gamma}$~ 30 $10^3$ $s^{-1}$ (Wi = 18.7, Q = 33 µl/min) as shown in Figure 1c. Such high shear rates can be easily reached in pathological cases like stenosis [5]. The vortices observed with the $PEO50_{15/85\text{-}Hct50}$ differ from the ones with the polymer solutions such as $PEO500_{15/85}$. For the latter, the vortices appear asymmetrically on the left and right sides of the channel but cover roughly its entire width; these vortices are also time dependent at high shear rates. For the case of the red blood cell polymer mixture, the vortices appear close to the inlet of the small channel and they grow at higher Weissenberg numbers over the whole width of the channel. For a given flow rate, they are stationary in time.

Finally we test full blood in the geometry but again we could not find any flow instability at any shear rate. We do not have a clear explanation for this, but there are still rheological differences between blood and the $PEO50_{15/85\text{-}Hct50}$ solution.

[1] L. E. Rodd, T. P. Scott, D. V. Boger, J. J. Cooper-White, and G. H. McKinley, J. Non-Newtonian Fluid Mech. 129, 1 (2005).

[2] L. E. Rodd, J. J. Cooper-White, D. V. Boger, and G. H. McKinley, J. Non-Newtonian Fluid Mech. 143, 170 (2007).

[3] Z. Li, X.-F. Yuan, S. J. Haward, J. A. Odell, and S. Yeates, Rheol. Acta 50, 277 (2011).

[4] A. Lanzaro and X.-F. Yuan, J. Non-Newtonian Fluid Mech. 166, 1064 (2011).

[5] N. Korin, M. Kanapathipillai, B. D. Matthews, M. Crescente, A. Brill, T. Mammoto, K. Ghosh, S. Jurek, S. A. Bencherif, D. Bhatta, A. U. Coskun, C. L. Feldman, D. D. Wagner, D. E. Ingber, Science 10, 738 (2012).

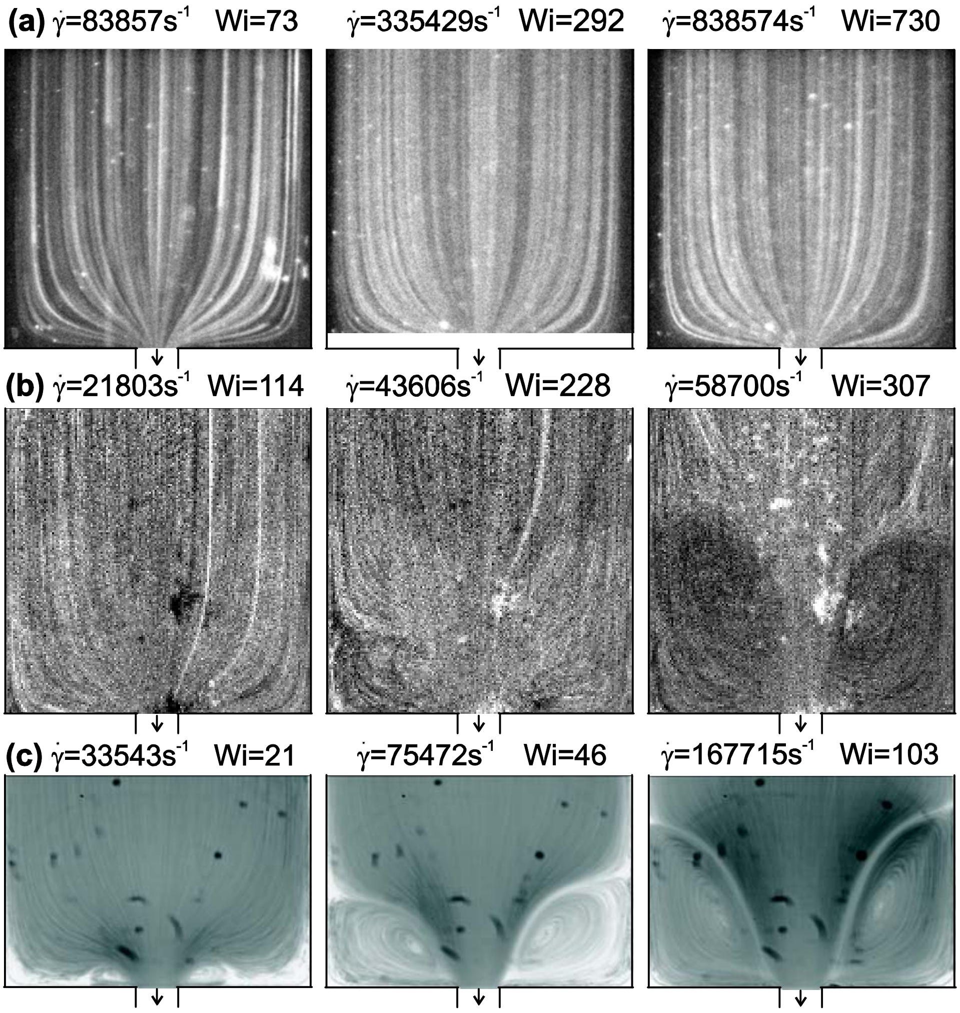


Fig 1: a) Streak images of plasma flowing through the contraction microfluidics. The images show the region upstream of the inflow into the contraction. For all shear rates no vortices could be observed. b) The PEO500$_{15/85}$ solution. In the first image the flow is still stable but in the second image on the left side a vortex is visible. c) The PEO50$_{15/85\text{-}Hct50}$ solution with upstream vortices that grow with increasing shear rate.
